# Supplementary material for: Investigation and Evaluation of Adaptive Algorithms for Multichannel Active Noise Control System
Source: arXiv:2308.15485 source file (2023-08-09)
Supplement: Supplementary file 1 [file appendix.tex]

% %=== APPENDIX ===

% \begin{appendices}
% \label{cha:appendices}

% \chapter{Introduction of Appendix}
% \markboth{Appendix A}{} % For appendix first (affects header)
% \begin{spacing}{1.5}

% The Appendix contains related data not necessary to the immediate understanding of the discussion in the report. This may contain materials such as: tables, graphs, illustrations, description of equipment, samples of forms, data sheets, questionnaires, equations, and any material that must be included for record purposes.
% Each entry (sample forms, detailed data for references, tables, pictures, questionnaires, charts, maps, graphic representations) in the appendix requires an identifying title. Every entry in the appendix must be referred to in the body of the report. Each appendix must be lettered, beginning with Appendix A. The list of appendices should be appearing in the table of contents following the list of references entry.

% \end{spacing}

% \chapter{Sample Code}
% \markboth{Appendix B}{} % For appendix second, etc.. 

% below shows how to insert highlighted source code from the source file.

% \inputminted[
% tabsize=4, % change this to set the spacing of tab
% breaklines, % automatically wrap the code
% fontsize=\scriptsize % Can be \footnotesize, \small, \normalsize etc
% ]{python}{Appendix/sample.py}

% \end{appendices}
